# Supplementary material for: Position-Blind Ptychography: Viability of image reconstruction via data-driven variational inference
Source: arXiv:2509.25269 source file (2026-05-29)
Supplement: Supplementary file 1 [file supplement.tex]

% SIAM Supplemental File Template
\documentclass[review,supplement,onefignum,onetabnum]{siamonline250211}

\input{ex_shared}

%\externaldocument[]{main}

% Optional PDF information
% \ifpdf
% \hypersetup{
%   pdftitle={Supplementary Materials: An Example Article},
%   pdfauthor={D. Doe, P. T. Frank, and J. E. Smith}
% }
% \fi

\begin{document}

\maketitle

\input{sections/95appendix}

\bibliographystyle{siamplain}
\bibliography{references}

\end{document}
